# Supplementary material for: Preservation of Feature Stability in Machine Learning Under Data Uncertainty for Decision Support in Critical Domains
Source: arXiv:2401.11044 source file (2024-08-06)

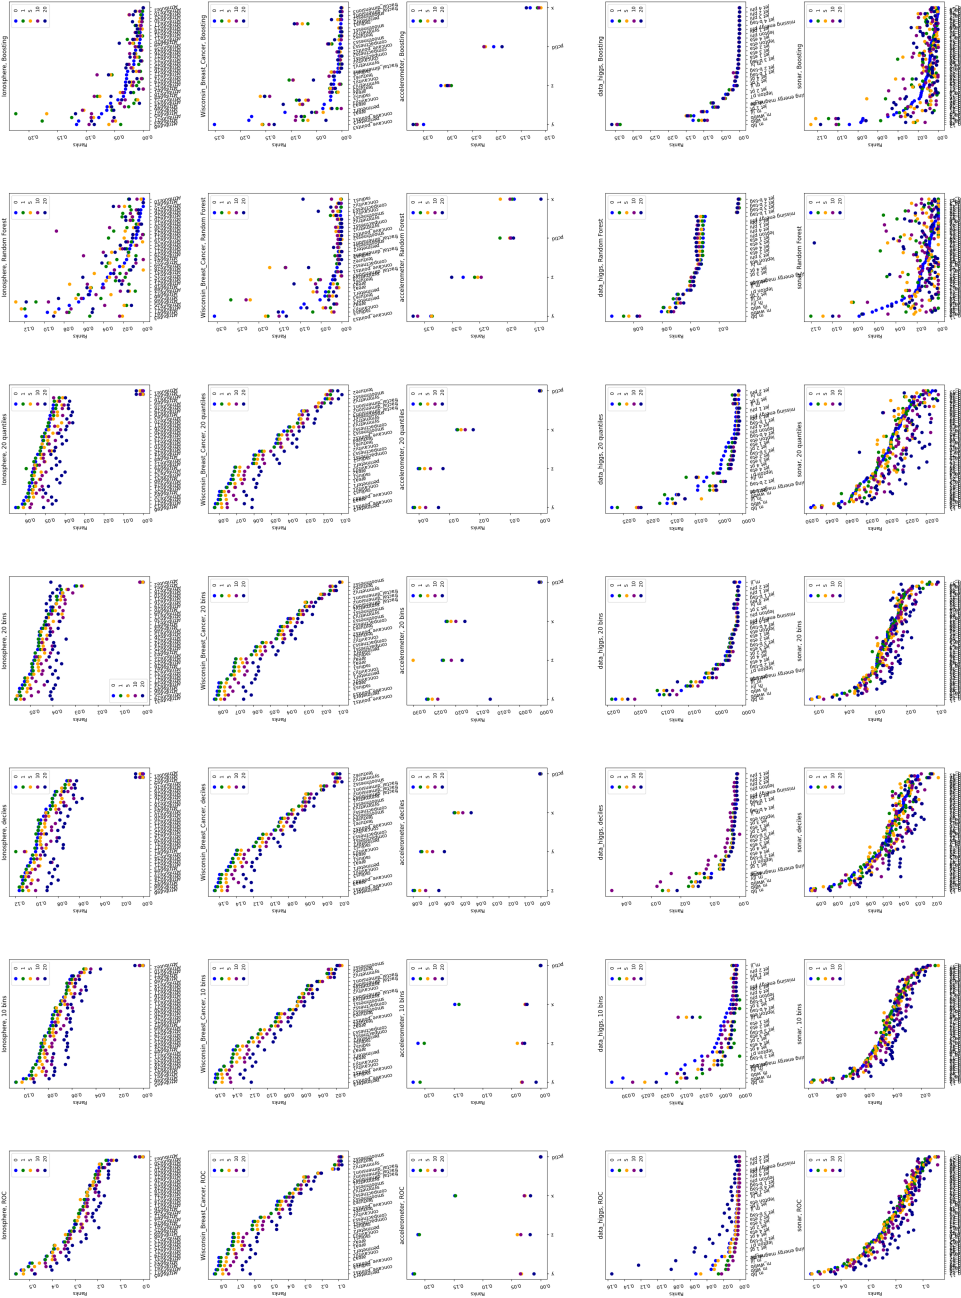

Figure S1: Feature significance of the different features. Different columns corresponds to the different ML methods SaNDA with different abstraction methods, RF and XGBoost respectively. Every row represent different dataset.

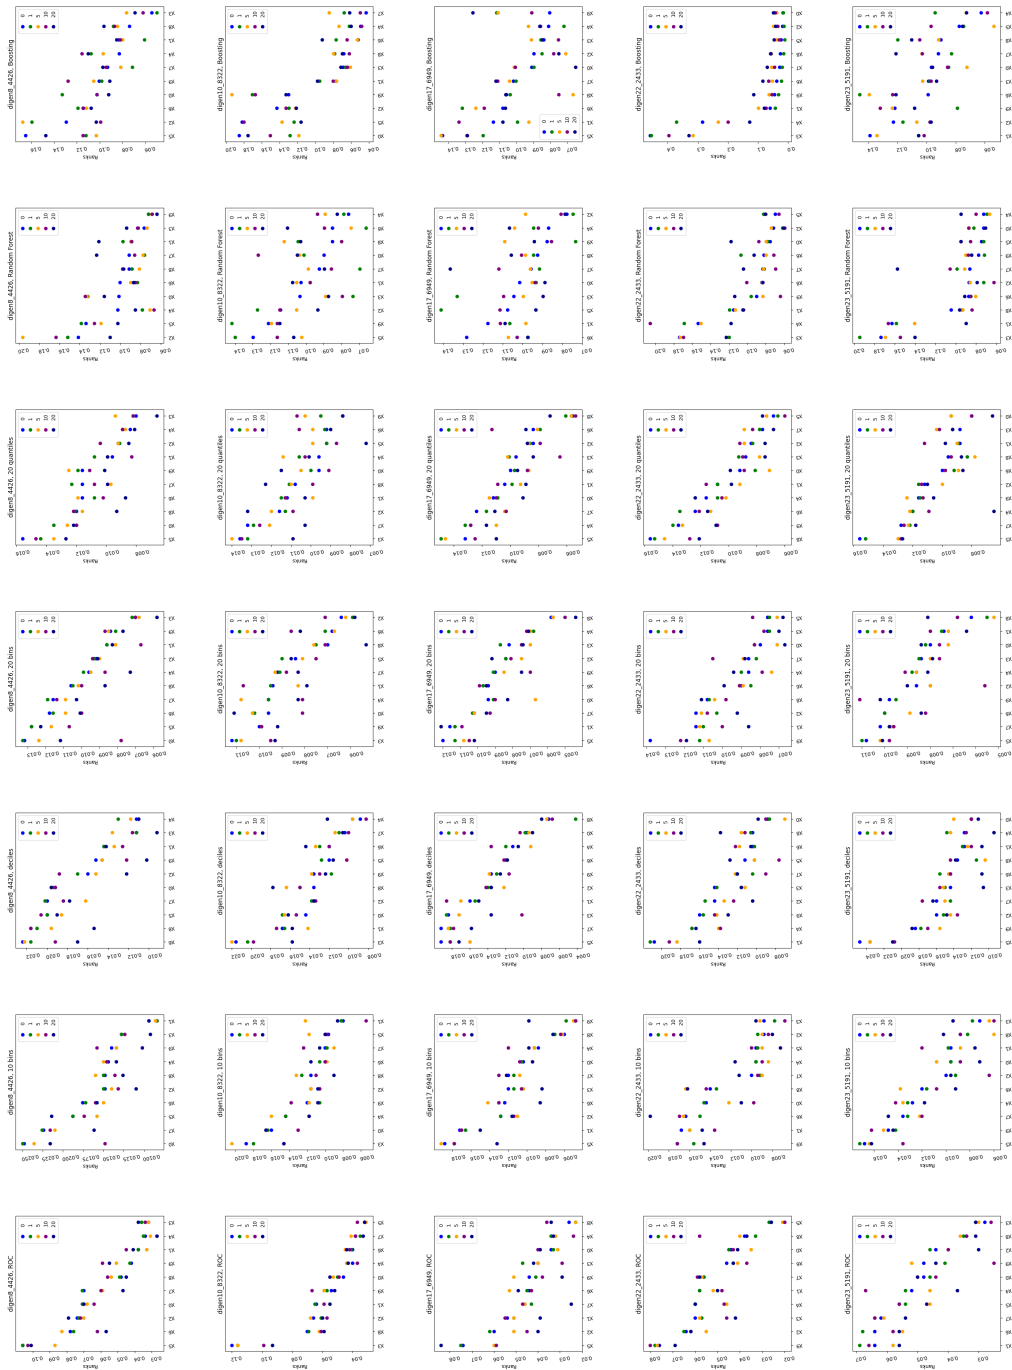

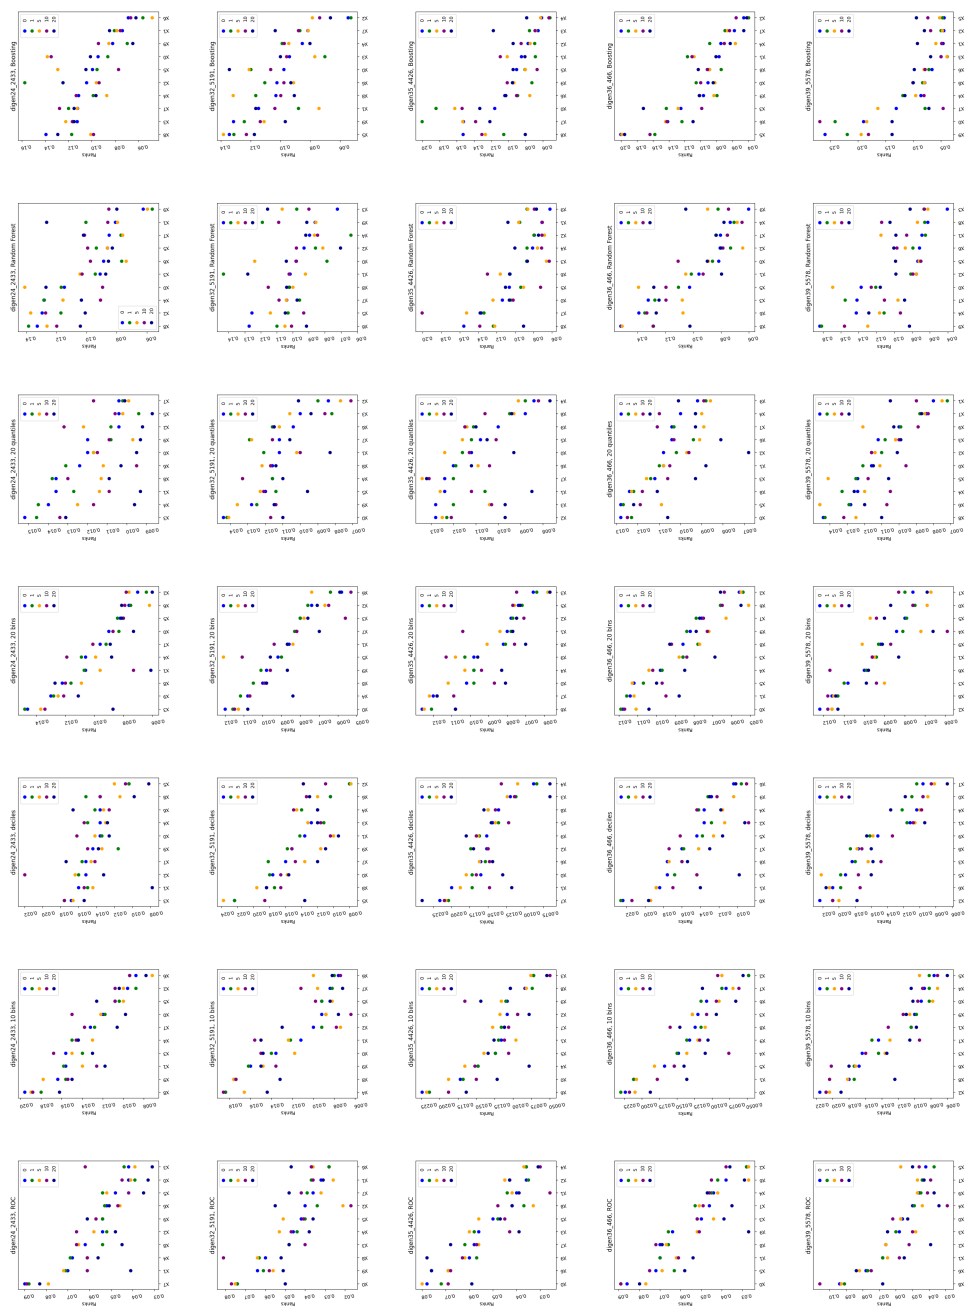

Supplement: Supplementary file 1 [file SM.pdf]
